# Supplementary material for: DO-Conv: Depthwise Over-parameterized Convolutional Layer
Source: arXiv:2006.12030 source file (2020-06-22)
Supplement: Supplementary file 1 [file 08_appendix.tex]

\appendix

\section{Equivalence between the feature and kernel composite}
\label{sec:proof}

\begin{proof}
%\begin{equation*}
\begin{align*}
    \mathbb{O}_{c_{out}} 
     &= \sum_{i}^{D_{mul} \times C_{in}} \mathbb{W}_{c_{out}i} \mathbb{P'}_{i} \tag{feature composite} \\
     &= \sum_{k}^{D_{mul}} \sum_{l}^{C_{in}} \mathbb{W}_{c_{out}kl} \mathbb{P'}_{kl}\\
    &= \sum_{k}^{D_{mul}} \sum_{l}^{C_{in}} \mathbb{W}_{c_{out}kl} (\sum_{j}^{M \times N} \mathbb{D}_{jkl} \mathbb{P}_{jl})\\
    &=\sum_{j}^{M \times N} \sum_{l}^{C_{in}} (\sum_{k}^{D_{mul}} \mathbb{D}^{T}_{kjl} \mathbb{W}_{c_{out}kl}) \mathbb{P}_{jl}\\
    &=\sum_{j}^{M \times N} \sum_{l}^{C_{in}} \mathbb{W'}_{c_{out}jl} \mathbb{P}_{jl}\\
    &=\sum_{i}^{(M \times N) \times C_{in}} \mathbb{W'}_{c_{out}i} \mathbb{P}_{i} \tag{kernel composite}
\end{align*}
%\end{equation*}
\label{pf:expressiveness}
\end{proof}
